# Supplementary material for: Superconducting switch for fast on-chip routing of quantum microwave fields
Source: arXiv:1606.01031 ancillary file (2016-06-03)
Supplement: Supplementary file 1 [file supplementary.pdf]

# Supplementary material for: Superconducting switch for fast on-chip routing of quantum microwave fields

M. Pechal,* J.-C. Besse, M. Mondal, M. Oppliger, S. Gasparinetti, and A. Wallraff
*Department of Physics, ETH Zurich, CH-8093 Zurich, Switzerland*
(Dated: June 3, 2016)

PACS numbers: 85.25.Cp

## I. MODEL OF THE RESONATOR FREQUENCY DEPENDENCE ON THE BIAS COIL VOLTAGE

To calculate the dependence of the resonator frequencies on the applied magnetic flux, we use the following model: The fundamental resonance frequency of the tunable resonator is a function of the SQUID array inductance $L$ and the capacitances $C_c$ coupling the resonator to the feedlines. The symmetry of the resonator with respect to its center implies that the fundamental mode has a voltage node at the center point. Therefore, for the purposes of further circuit analysis, we can connect this point to ground and analyze only one of the two halves of the resulting circuit (see Fig. 1).

The resonance frequency can be determined by expressing the admittance of the circuit as a function of frequency and finding its zero. The node at which the admittance is taken can be chosen arbitrarily as long as the mode of interest has a non-zero voltage amplitude there. Here we choose the node at the end of the resonator indicated in Fig. 1 by $\times$. The admittance is found to be

$$Y = \frac{\mathrm{i}}{Z_0}\left(\frac{x_c\delta}{\mathrm{i}x_c\delta+1} - \frac{1-x_L\delta\tan\delta}{x_L\delta+\tan\delta}\right),$$

where $\delta = \omega l/2v$ is the phase accumulated by the signal upon propagation over a distance $l/2$, half the length of the resonator, $v$ is the propagation velocity in the transmission line and $x_c = 2vC_cZ_0/l$, $x_L = vL/Z_0 l$ are dimensionless parameters quantifying the coupling capacitance $C_c$ and the SQUID array inductance $L$. Equating $Y$ to zero gives us the resonance condition

$$\tan\delta = \mathrm{i} + \frac{1}{\delta}\frac{1-\mathrm{i}x_L\delta}{x_c+x_L+\mathrm{i}x_c x_L\delta} \tag{1}$$

which takes a particularly simple form (cf. Ref. [1]) in the limit $C_c = 0$:

$$\delta\tan\delta = \frac{1}{x_L}.$$

Specifically, for $L = 0$ we get $\delta = \pi/2$ at the bare resonance frequency $\omega_{r0}$ and therefore $\delta$ can be expressed in terms of frequency as $\delta = \pi\omega/2\omega_{r0}$. The relation between the resonance frequency $\omega_r$ and the SQUID array inductance $L$ is then

$$\tan\frac{\pi\omega_r}{2\omega_{r0}} = \frac{2Z_0}{\omega_r L}. \tag{2}$$

A measurement of the resonance frequency in a resonator sample where the SQUID array is replaced by a short niobium wire yields the bare frequency $\omega_{r0}/2\pi = 8.3\,\mathrm{GHz}$. Eq. (2) then allows us to calculate the SQUID array inductances $L$ corresponding to the resonance frequencies extracted as a function of the voltage $V$ applied to the flux bias coil.

In its linear regime, an asymmetric SQUID loop can be approximated as a variable inductor whose inductance can be tuned by an applied magnetic flux between its minimum and maximum value $L_{\min}$ and $L_{\max}$. The inductance is given by

$$L_S(\phi) = \frac{L_{\min}L_{\max}}{\sqrt{L_{\max}^2\cos^2\frac{\phi}{2} + L_{\min}^2\sin^2\frac{\phi}{2}}},$$

where $\phi$ is related to the magnetic flux $\Phi$ threading the loop and the magnetic flux quantum $\Phi_0$ by $\phi = 2\pi\Phi/\Phi_0$.

We assume that the Josephson energies of the junctions comprising the five individual SQUID loops in the array are identical but we allow for the possibility that the fluxes $\Phi_1,\ldots,\Phi_5$ threading the loops are unequal. However, we will constrain them to satisfy $\Phi_1 = \Phi_5$ and $\Phi_2 = \Phi_4$ due to symmetry of the sample. We will further take the fluxes to be linear functions of the applied coil voltage $V$ of the form $\Phi_1 = \Phi_5 = \Phi_0(V - V_0)/V_1$, $\Phi_2 = \Phi_4 = \Phi_0(V - V_0)/V_2$ and $\Phi_3 = \Phi_0(V - V_0)/V_3$.

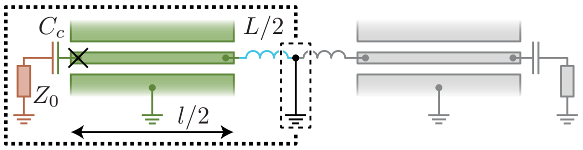


FIG. 1. Schematic diagram of the tunable resonator. For calculation of the fundamental mode frequency, the center point is connected to ground, as indicated in the dashed box. The dotted box shows the reduced circuit whose resonance frequency is to be found. The node chosen for the admittance calculation is marked by $\times$.

* mpechal@phys.ethz.ch

The total inductance of the SQUID array is then

$$\begin{aligned}L(V) =& 2L_S(2\pi(V-V_0)/V_1)\\ &+2L_S(2\pi(V-V_0)/V_2)\\ &+L_S(2\pi(V-V_0)/V_3).\end{aligned}$$

We fit this function to the inductances calculated from the measured resonance frequencies, treating $V_0$, $V_1$, $V_2$, $V_3$, $L_{\min}$ and $L_{\max}$ as fit parameters. For the data shown in this paper, the optimal fit is found for $V_0 = 0.984\,\mathrm{V}$, $V_1 = 3.192\,\mathrm{V}$, $V_2 = 3.686\,\mathrm{V}$, $V_3 = 3.686\,\mathrm{V}$, $L_{\min} = 0.064\,\mathrm{nH}$ and $L_{\max} = 0.354\,\mathrm{nH}$. These inductances correspond to Josephson energies of 2.55 THz and 0.46 THz, respectively.

The fitted dependence $L(V)$ is then used to calculate $\omega_r(V)$ using Eq. (2). The result is shown in Fig. 3(a) of the main text as a curve on top of the density plot of the transmission coefficent as a function of the coil voltage and signal frequency. The agreement between the measurement and the fit shows that we have a good understanding of the flux dependence of the resonator frequencies.

## II. DIGITAL PROCESSING OF THE SIGNAL

To acquire the data in the continuous tone measurements, we use a Virtex 4 field-programmable-gate-array (FPGA) equipped with an analog-to-digital converter (ADC) with a sampling rate of 100 MS/s. The preamplified signal, down-converted to an intermediate frequency of 25 MHz, is digitized and further processed by the FPGA. This processing consists of multiplication by a complex 25 MHz signal $s_j = \exp(-\mathrm{i}\pi j/2)$, followed by averaging in the FPGA.

In the large bandwidth measurements performed to observe the switching waveforms, we use a Virtex 6 FPGA with a 1 GS/s analog-to-digital converter. Here, the digitized waveforms are averaged and their mean is recorded without any further processing by the FPGA. All subsequent data analysis is then done in software. After digital down-conversion of the signal from its intermediate frequency of 250 MHz to dc, we convolve it with a filter which has a sinc shape in time domain. This corresponds to a boxcar function in the frequency domain, centered around zero with a width of 500 MHz. Such a filter therefore removes all frequency components above 250 MHz. In addition, to remove artifacts of the digital processing attributed to cross-talk of digital signals in the FPGA, we explicitly set frequency components at 250 and 125 MHz to zero.

## III. NON-LINEARITY OF THE SWITCH

Here we present the derivation of the non-linearity of the resonator [2, 3] and the 1 dB compression point of the switch device. For a more detailed discussion of non-linear effects in resonators with embedded arrays of Josephson junctions, we refer the reader to Ref. [1].

We describe the tunable resonator as a Duffing oscillator with a Hamiltonian

$$H/\hbar = \omega_r a^\dagger a + \frac{1}{2}K a^\dagger a^\dagger a a, \tag{3}$$

where the Kerr non-linearity $K$ is the lowest-order anharmonic correction to the resonator energy levels due to the non-linearity of the Josephson junctions. We will study the case when the resonators are driven resonantly. In a rotating frame at the signal frequency $\omega_s = \omega_r$, the input-output relations for the resonator probed in transmission are

$$\begin{aligned}\dot{a} &= -\mathrm{i}K a^\dagger a a + \sqrt{\frac{\kappa}{2}} a_{\mathrm{in}} - \frac{\kappa}{2} a,\\ b_{\mathrm{out}} &= \sqrt{\frac{\kappa}{2}} a.\end{aligned}$$

In the classical approximation, we replace the operators $a$ and $b$ by $c$-numbers $\alpha$ and $\beta$ and get the steady state equations

$$\alpha = \frac{\sqrt{\frac{\kappa}{2}}\alpha_{\mathrm{in}}}{\mathrm{i}K|\alpha|^2 + \frac{\kappa}{2}} = \beta_{\mathrm{out}}\sqrt{\frac{2}{\kappa}}.$$

Its solution can be found to lowest order in $K$ as

$$\frac{\beta_{\mathrm{out}}}{\alpha_{\mathrm{in}}} = \frac{1}{\frac{4\mathrm{i}K|\alpha_{\mathrm{in}}|^2}{\kappa^2} + 1}.$$

Therefore, the power transmission is suppressed by 1 dB, that is, a factor of $\epsilon = 10^{1/10}$ when $16K^2|\alpha_{\mathrm{in}}|^4/\kappa^4 + 1 = \epsilon$. The power $P_{\mathrm{cp}} = 2\hbar\omega_r|\alpha_{\mathrm{in}}|^2$ entering the switch at its 1 dB compression point is then given by

$$P_{\mathrm{cp}} = \frac{\hbar\kappa^2\omega_r\sqrt{\epsilon - 1}}{2|K|}. \tag{4}$$

To calculate the Kerr non-linearity $\hbar K$, we first notice that it is by definition (see Eq. (3)) equal to $\mathrm{d}^2E_n/\mathrm{d}n^2$, where $E_n$ are the energy levels of the non-linear oscillator. The Hamiltonian of the circuit is given by

$$H = H_{\mathrm{TL}} + NE_J(1 - \cos(\varphi/N)),$$

where $H_{\mathrm{TL}}$ is the Hamiltonian of the circuit excluding the SQUID loop array, $E_J$ is the Josephson energy of each of the $N$ individual SQUIDs and $\varphi$ the phase drop across the array. We expand the cosine to fourth order in $\varphi$ and group the quadratic term $E_J\varphi^2/2N$ together with $H_{\mathrm{TL}}$ into $H_{\mathrm{lin}}$, a Hamiltonian of a linearized circuit where the SQUID array has been approximated by an inductor of inductance $L = N\Phi_0^2/4\pi^2E_J$. In the last equation, $\Phi_0$ denotes the magnetic flux quantum $h/2e$. The circuit Hamiltonian including the quartic term in $\varphi$ is then

$$H = H_{\mathrm{lin}} - \frac{1}{24N^2L}\left(\frac{\Phi_0}{2\pi}\right)^2\varphi^4.$$

We can express the phase drop $\varphi$ in terms of the ladder operators $a$ and $a^\dagger$ as $\varphi = \varphi_{\mathrm{vac}}(a+a^\dagger)$. The lowest-order anharmonic correction to the resonator energy levels is therefore given by

$$\Delta E_n = -\frac{\varphi_{\mathrm{vac}}^4}{24N^2L}\left(\frac{\Phi_0}{2\pi}\right)^2 \langle n|(a+a^\dagger)^4|n\rangle,$$

which then yields

$$\hbar K = \frac{\mathrm{d}^2}{\mathrm{d}n^2}\Delta E_n = -\frac{\varphi_{\mathrm{vac}}^4}{2N^2L}\left(\frac{\Phi_0}{2\pi}\right)^2.$$

We can express the vacuum amplitude of the phase drop $\varphi_{\mathrm{vac}}$ by considering the fraction $E_{L,\mathrm{vac}}$ of the vacuum energy $E_{\mathrm{vac}} = \hbar\omega_r/2$ stored in the SQUID array

$$\frac{E_{L,\mathrm{vac}}}{E_{\mathrm{vac}}} = \frac{2}{\hbar\omega_r}\langle 0|\frac{\varphi^2}{2L}\left(\frac{\Phi_0}{2\pi}\right)^2|0\rangle = \frac{\varphi_{\mathrm{vac}}^2}{\hbar\omega_r L}\left(\frac{\Phi_0}{2\pi}\right)^2.$$

This can be used to transform the expression for $K$ into the form

$$K = -\left(\frac{E_{L,\mathrm{vac}}}{E_{\mathrm{vac}}}\right)^2\frac{2\omega_r^2e^2L}{\hbar N^2}.$$

By straightforward classical analysis of the resonator circuit, we calculate the relative fraction of its energy stored in the inductor. For the sake of simplicity, we work in the approximation of vanishing coupling capacitance. The obtained energy fraction is independent of the total energy stored in the circuit and is also equal to the ratio $E_{L,\mathrm{vac}}/E_{\mathrm{vac}}$.

$$\frac{E_L}{E} = \frac{1}{1+(y+1/y)\arctan y},$$

where $y = 2Z_0/\omega_r L$. According to Eq. (2), for a $\lambda/2$ resonator, this parameter can be also expressed as $\tan(\pi\omega_r/2\omega_{r0})$. The resulting expression for $K$ is

$$K = -\frac{\omega_r}{N^2}\frac{4Z_0e^2}{\hbar}\frac{1}{y(1+(y+1/y)\arctan y)^2}, \qquad (5)$$

which after substitution into Eq. (4) yields the following expression for the input power at the 1 dB compression point:

$$P_{\mathrm{cp}} = \frac{\hbar^2\kappa^2N^2\sqrt{\epsilon-1}}{8Z_0e^2}y(1+(y+1/y)\arctan y)^2. \qquad (6)$$

This equation gives us a theoretical estimate of the device's 1 dB compression point based on its linear parameters. As discussed in the main text of the manuscript, the obtained estimate of −81 dBm agrees reasonably well with the measured 1 dB compression point at −86 dBm and the difference is attributed mainly to the reduction in loss of the microwave lines with temperature.

## IV. ANALYSIS OF PHOTON STATES

To determine the state of the detected field $a$, we use a method described in Ref. [4] where the density matrix is obtained by a maximum likelihood method from a set of moments $\langle (a^\dagger)^i a^j\rangle$. Up to a scaling factor, the measured heterodyne voltage can be described as an observable with an operator $S = a + h^\dagger$ where $h$ is a harmonic mode describing the added noise in the detection process. We record each single-shot measurement of the voltage in a histogram which allows us to calculate moments of the form $\langle (S^\dagger)^i S^j\rangle$. These can be expressed as sums of terms such as $\langle (a^\dagger)^k a^l\rangle\langle h^m (h^\dagger)^n\rangle$.

In the absence of the signal, that is, if $\langle (a^\dagger)^i a^j\rangle = 0$ for any $i, j$, the measured moments $\langle (S^\dagger)^i S^j\rangle_0$ directly yield the noise moments $\langle h^i (h^\dagger)^j\rangle$. From a set of measurements with the signal on and off, we can then systematically reconstruct the signal moments $\langle (a^\dagger)^i a^j\rangle$. For example, the moments $\langle a\rangle$ and $\langle a^\dagger a\rangle$ can be expressed as

$$\begin{aligned}\langle a\rangle &= \langle S\rangle - \langle S\rangle_0,\\ \langle a^\dagger a\rangle &= \langle S^\dagger S\rangle - \langle S^\dagger S\rangle_0 - 2\mathrm{Re}(\langle S\rangle - \langle S\rangle_0)\langle S^\dagger\rangle_0.\end{aligned}$$

The scaling factor between the measured voltage and $S$ needs to be calibrated using a measurement where at least one of the moments is known. For this purpose, we collected the histograms and calculated the moments for a series of photon states prepared by exciting the transmon with pulses of varying amplitude $A$. A resonant preparation pulse rotates the Bloch vector describing the qubit state by an angle $\theta \propto A$ around an axis lying in the equatorial plane of the Bloch sphere. The prepared qubit state is $\cos(\theta/2)|g\rangle + \mathrm{e}^{\mathrm{i}\phi}\sin(\theta/2)|e\rangle$ which, after the qubit spontaneously relaxes, results in the photon state $|\psi\rangle = \cos(\theta/2)|0\rangle + \mathrm{e}^{\mathrm{i}\phi}\sin(\theta/2)|1\rangle$. The corresponding expectation values $\langle a\rangle$ and $\langle a^\dagger a\rangle$ are

$$\begin{aligned}\langle a\rangle &= \frac{1}{2}\mathrm{e}^{\mathrm{i}\phi}\sin\theta,\\ \langle a^\dagger a\rangle &= \sin^2\frac{\theta}{2}.\end{aligned}$$

We further take into account that dephasing of the qubit can lead to a reduction of the coherent signal $\langle a\rangle$ by some factor $k < 1$. We denote the proportionality factor between the rotation angle $\theta$ and the applied pulse amplitude by $c = \theta/A$ and the scaling factor relating the measured voltage $V$ to $S$ by $\lambda = S/V$. The expected relation between the moments of $V$ and the pulse amplitude $A$ is therefore

$$\lambda|\langle V\rangle - \langle V\rangle_0| = \frac{1}{2}k|\sin cA|,$$

$$\begin{aligned}\lambda^2(\langle V^\dagger V\rangle - \langle V^\dagger V\rangle_0 - &2\mathrm{Re}(\langle V\rangle - \langle V\rangle_0)\langle V^\dagger\rangle_0 =\\ &= \sin^2\frac{cA}{2}.\end{aligned}$$

We fit these dependences to the measured moments to obtain the unknown parameters $\lambda$, $\kappa$ and $c$. We then verify our measurement and analysis by plotting the extracted moments of $a$ as a function of the rotation angle $\theta$ and comparing them with the theory. The plot in Fig. 6(b) of the main text shows a good match of the extracted moments with theory, indicating that our single photon source as well as the analysis procedure work as expected.

To obtain the Wigner function of the measured photon state, we first extract its density matrix $\rho$ using a maximum likelihood method [4]. Here the density matrix is parametrized as $\rho(M) = M^\dagger M / \mathrm{Tr}\, M^\dagger M$, where $M$ is an upper triangular matrix with real elements on the diagonal [5]. This parametrization automatically ensures that $\rho(M)$ is positive semi-definite and its trace is unity. The elements of $M$ are then chosen to minimize the deviations of the measured moments from their predicted values $\mathrm{Tr}\, \rho(M)(a^\dagger)^i a^j$. The cost function $f$ for this minimization is chosen as

$$f(M) = \sum_{i,j} \frac{1}{\sigma_{ij}^2} |\langle (a^\dagger)^i a^j \rangle - \mathrm{Tr}\, \rho(M)(a^\dagger)^i a^j|^2,$$

where $\sigma_{ij}$ are the uncertainties of the individual moments. In our analysis, $M$ and therefore also $\rho$ are restricted to be $6 \times 6$ matrices and only moments $\langle (a^\dagger)^i a^j \rangle$ for $i + j \leq 6$ are used in the calculation. Thus we implicitly assume that no more than the lowest six Fock states are occupied. This assumption is justified by the fact that the moment $\langle a^\dagger a^\dagger a a \rangle$ puts an upper bound on the total occupation $p_{\geq n}$ of all Fock states with more than $n$ photons: $p_{\geq n} \leq \langle a^\dagger a^\dagger a a \rangle / n(n+1)$.

The optimal density matrix is then used to calculate the Wigner function using the formula [6]

$$W(\alpha) = 2\mathrm{Tr}\, \mathrm{e}^{\alpha^* a - \alpha a^\dagger} \rho \mathrm{e}^{-\alpha^* a + \alpha a^\dagger} P,$$

where $P$ is the parity operator and $a$ the annihilation operator restricted to the subspace with fewer than six photons.


[1] C. Eichler and A. Wallraff, EPJ Quantum Technology **1**, 2 (2014).

[2] P. Bertet, F. R. Ong, M. Boissonneault, A. Bolduc, F. Mallet, A. C. Doherty, A. Blais, D. Vion, and D. Esteve, "Circuit quantum electrodynamics with a nonlinear resonator," arXiv:1111.0501v1 [quant-ph] (2011), 1111.0501 [quant-ph].

[3] M. Dykman, ed., *Fluctuating Nonlinear Oscillators* (Oxford University Press, 2012).

[4] C. Eichler, D. Bozyigit, and A. Wallraff, Phys. Rev. A **86**, 032106 (2012).

[5] D. F. V. James, P. G. Kwiat, W. J. Munro, and A. G. White, Phys. Rev. A **64**, 052312 (2001).

[6] K. E. Cahill and R. J. Glauber, Phys. Rev. **177**, 1882 (1969).
